# Supplementary material for: Robust formation of nanoscale magnetic skyrmions in easy-plane thin film multilayers with low damping
Source: arXiv:2102.11117 ancillary file (2021-02-22)
Supplement: Supplementary file 1 [file Supplemental_Information.pdf]

# Supplementary Information: Robust formation of nanoscale magnetic skyrmions in easy-plane thin film multilayers with low damping

Luis Flacke,<sup>1,2,\*</sup> Valentin Ahrens,<sup>3</sup> Simon Mendisch,<sup>3</sup> Lukas Körber,<sup>4,5</sup> Tobias Böttcher,<sup>6</sup> Elisabeth Meidinger,<sup>1,2</sup> Misbah Yaqoob,<sup>1,2</sup> Manuel Müller,<sup>1,2</sup> Lukas Liensberger,<sup>1,2</sup> Attila Kákay,<sup>4</sup> Markus Becherer,<sup>3</sup> Philipp Pirro,<sup>6</sup> Matthias Althammer,<sup>1,2</sup> Stephan Geprägs,<sup>1</sup> Hans Huebl,<sup>1,2,7</sup> Rudolf Gross,<sup>1,2,7</sup> and Mathias Weiler<sup>1,2,6,†</sup>

<sup>1</sup>Walther-Meißner Institut, Bayerische Akademie der Wissenschaften, 85748 Garching, Germany

<sup>2</sup>Physics Department, Technical University of Munich, 85748 Garching, Germany

<sup>3</sup>Chair of Nano and Quantum Sensors, Technical University of Munich, 80333 Munich, Germany

<sup>4</sup>Helmholtz-Zentrum Dresden-Rossendorf e.V., Institute of Ion Beam Physics and Materials Research, 01328 Dresden, Germany

<sup>5</sup>Fakultät Physik, Technische Universität Dresden, 01062 Dresden, Germany

<sup>6</sup>Fachbereich Physik and Landesforschungszentrum OPTIMAS,  
Technische Universität Kaiserslautern, 67663 Kaiserslautern, Germany

<sup>7</sup>Munich Center for Quantum Science and Technology (MCQST), 80799 Munich, Germany

(Dated: February 18, 2021)

## SAMPLES AND FABRICATION

The samples were fabricated by magnetron sputter deposition on thermally oxidized Si (001) substrates at an Ar pressure of  $5 \times 10^{-3}$  mbar at room temperature. The base pressure of the vacuum chamber is  $10^{-9}$  mbar. The sample discussed in the main text consisted of Ta(1.5)/Pt(6)/Cu(3) seed layers, followed by the sixfold repeated trilayer [Pt(0.6)/Co<sub>25</sub>Fe<sub>75</sub>(1.1)/Ir(0.7)]<sub>6</sub> and a capping Cu(3)/Ta(1.5), where the numbers in parenthesis represent nominal layer thicknesses in nm. The Co<sub>25</sub>Fe<sub>75</sub>-alloy will be abbreviated as CoFe throughout the entire supplementary information.

Further reference samples were fabricated in order to determine the interface Dzyaloshinskii-Moriya (iDMI) strength by Brillouin Light Scattering (BLS) [1] and to exclude antiferromagnetic RKKY coupling contributions. Analogously to Zeissler *et al.* [2], the iDMI was determined using samples with single trilayers, as the DMI strength should not be affected by the number of repetitions. For the BLS measurements the set of samples consists of Pt(0.6)/CoFe( $t_{\text{CoFe}}$ )/Ir(0.7) with varying thickness  $t_{\text{CoFe}} = (0.95/1.1/1.5/2/3)$  nm of the CoFe layer and Pt( $t_{\text{Pt}}^{\text{BLS}}$ )/CoFe(1.1)/Ir(0.7) with different thicknesses  $t_{\text{Pt}}^{\text{BLS}} = (0.2/0.4/0.6/0.8/1)$  nm of the Pt layer. In order to study the sign of the RKKY coupling between repeated trilayers, two sets of sample series were fabricated with different Ir-thickness  $t_{\text{Ir}}$  Pt(0.75)/CoFe(1.1)/Ir( $t_{\text{Ir}}$ ) and different Pt-thickness  $t_{\text{Pt}}^{\text{RKKY}}$  Pt( $t_{\text{Pt}}^{\text{RKKY}}$ )/CoFe(1.1)/Ir(0.45), where  $t_{\text{Ir}}$  varies from 0 nm to 1 nm and  $t_{\text{Pt}}^{\text{RKKY}}$  varies from 0.4 nm to 0.9 nm. The seed layers of these additional samples consist of Ta(1.5)/Pt(4)/Cu(2), and the capping is Cu(2)/Ta(2.5).

## MAGNETIC FORCE MICROSCOPY AND RADIUS ANALYSIS

Magnetic force microscopy (MFM) images were obtained at ambient conditions and a distance of 20 nm between tip and sample surface. The magnetic field was adjusted by changing the position of a permanent magnet below the sample, leading to a field range between  $(66 \pm 6)$  mT and  $(309 \pm 15)$  mT. In order to determine the radius of skyrmions from the MFM images, a large number (28-115) of skyrmions was selected for data processing. The center position of individual skyrmions was determined from the MFM phase images and their radial profile was averaged over the azimuthal direction. In order to determine the apparent radius, the obtained radial profile is plotted vs. the radial distance and a Gaussian-fit was applied to the data as shown in Fig. 2 in the main text. Fig. S1 a) shows a MFM image, where the green dots represent the batch of selected skyrmions. Four skyrmions are highlighted in different color and are analyzed in Fig. S1 b), showing their respective radial profiles. The Gaussian fits agree well with the experimental data. (The center of the Gaussian was fixed to the origin). The radius  $r$  in the main text is the arithmetic mean and the  $y$ -error bar in Fig. 2 b) in the main text represents one standard deviation obtained from performing the described data processing for an ensemble of skyrmions for each value of  $\mu_0 H_{\text{ext}}$ . The corresponding histogram is shown in Fig. S1 c) which exhibits a normal distribution of the skyrmion radii.

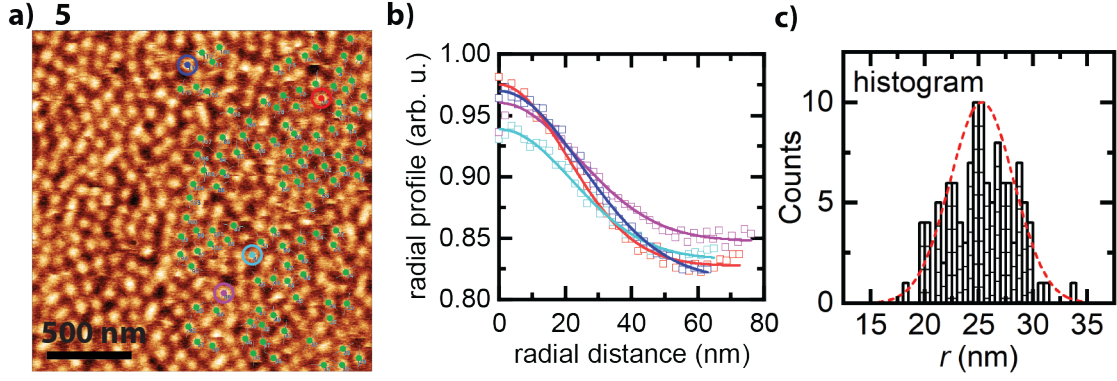

FIG. S1. a) The image is a copy of Fig. 1b) (5) from the main text. The green dots indicate the batch of selected skyrmions for the radius analysis. Four skyrmions are highlighted in a different color and their respective radial profile is plotted in b). The radial profiles in b) depict a Gaussian behavior and the apparent skyrmion radii were determined by the half width at half maximum value. The symbols show the experimental data, whereas the solid lines show the respective Gaussian fit. c) The corresponding radius histogram of the analyzed skyrmions. The dotted normal distribution curve serves as a guide to the eye.

### BRILLOUIN LIGHT SCATTERING

Brillouin Light Scattering was used to determine the iDMI on single trilayer reference samples [1, 2]. In the presence of DMI, the spin-wave dispersion exhibits a non-reciprocal frequency shift:

$$f_{\text{DMI}} = \frac{\gamma}{\pi M_s} D k. \quad (\text{S1})$$

Here,  $\gamma$  is the gyromagnetic ratio,  $M_s$  is the saturation magnetization,  $D$  represents the effective DMI strength and  $k$  is the wave vector. When measuring the two counter propagating spin waves a frequency shift is observed:

$$\Delta f = f(k) - f(-k) = 2 \cdot \frac{\gamma}{\pi M_s} D |k|. \quad (\text{S2})$$

In the experiment, this is realized by measuring the Stokes and anti-Stokes BLS signal. Additionally, we reverse the

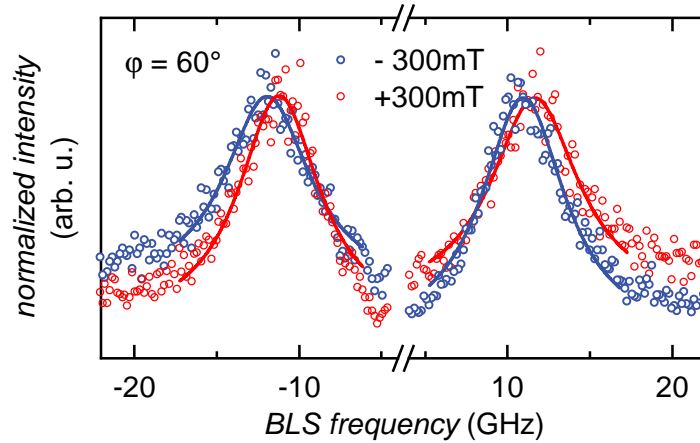

FIG. S2. Stokes and anti-Stokes peaks of the  $t_{\text{CoFe}} = 1.1$  nm sample in in-plane (IP) fields with an incident angle of  $\varphi = 60^\circ$  between light beam and surface normal. The DMI induces a frequency shift, which can be inverted by a sign change of the wave vector or by comparing Stokes and anti-Stokes peaks.

external magnetic field of  $\mu_0 H = 300$  mT to invert the direction of magnetization and observe the same frequency shift  $f(M, k) - f(-M, k) = \Delta f$  as shown in Fig. S2. The magnitude of the wave vector is set by the angle of incidence of the light relative to the film normal. In Fig. S2 we use  $\varphi = 60^\circ$  corresponding to  $|k| = 23.8 \text{ rad}/\mu\text{m}$ . The frequency shift depends linearly on the wave vector and, thus, can be tuned by the angle between incident light and sample surface

normal. We determine the DMI strength  $D$  by performing experiments as shown in Fig. S2 for  $13.7 \text{ rad}/\mu\text{m} \leq k \leq 25.8 \text{ rad}/\mu\text{m}$  and carrying out a linear fit to  $\Delta f$  vs  $k$ . The saturation magnetization  $M_S = 1112 \text{ kA/m}$  is obtained from the IP SQUID magnetometry measurement of the sample, the gyromagnetic ratio  $\gamma = 176 \times 10^9 \text{ rad}/(\text{Ts})$  is extracted from broadband magnetic resonance measurements as in Fig. S7. With Eq. (S2) we find  $D = (0.30 \pm 0.03) \text{ mJ/m}^2$ . By assuming an average lattice constant for CoFe from Ref. [3] with  $a = 0.32 \text{ nm}$ , we determine the DMI strength at the interface with [1]

$$D_{\text{int}} = t_{\text{CoFe}} \frac{\sqrt{3}}{a} D. \quad (\text{S3})$$

With the FM thickness of  $t_{\text{CoFe}} = 1.1 \text{ nm}$ , we obtain  $D_{\text{int}} = (1.86 \pm 0.19) \text{ mJ/m}^2$ , which aligns very well with the value in Ref. [4] on multilayers comprising the same used metals [4].

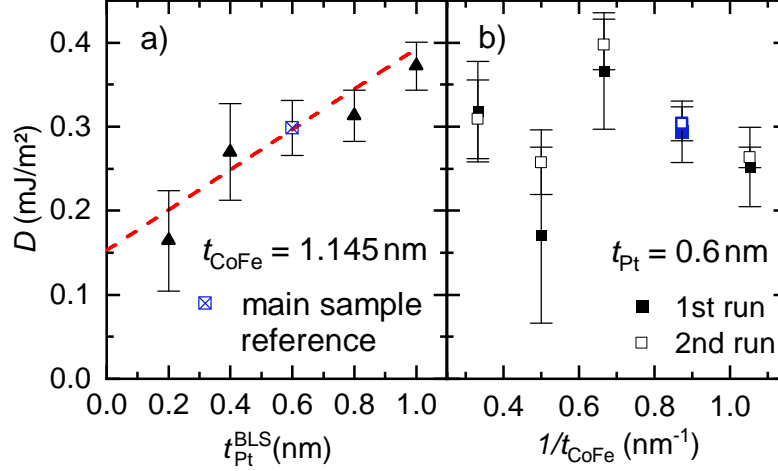

FIG. S3. The effective DMI strength was determined for two sets of sample series.  $D$  was calculated by employing  $M_S = 1112 \text{ kA/m}$  which was measured in a multilayer with  $t_{\text{CoFe}} = 1.1 \text{ nm}$ . a) The first series comprises a fixed FM layer and a varying Pt thickness. The red line is a guide to the eye, and the blue square corresponds to the sample measured in the second sample series presented in b). Here, the Pt thickness was fixed and the CoFe layer thickness was varied. Even though an interface induced linear behavior with  $1/t_{\text{CoFe}}$  is not observed, the reproducibility of the BLS measurements is confirmed by performing two separate runs of measurements of the sample series.

The determined effective DMI  $D$  of the different samples of the two sample series with varying Pt and CoFe thicknesses are presented in Fig. S3. The first set - variation of Pt thickness - exhibits an increasing  $D$  value with rising Pt thickness. Within the sub nm regime, a full Pt coverage of the surface is not expected [5]. Thus, an increasing thickness would correspond to an increased surface coverage leading to higher DMI contributions at the interface. As interface effects scale with the reciprocal thickness,  $D$  should also increase linearly with  $1/t_{\text{CoFe}}$ . Fig. S3 b) shows no clear trend which is attributed to the fact that within this ultra-thin regime material parameters such as Heisenberg exchange can change strongly with the FM thickness [1]. The largest volume-averaged DMI strength is obtained for  $t_{\text{CoFe}} = 1.5 \text{ nm}$ . This implies that ultrathin samples ( $t_{\text{CoFe}} < 1 \text{ nm}$ ) are not required to maximize DMI strength in this approach. The reproducibility of the presented results is demonstrated by running two separate sets of measurements on the sample series. All the values were determined by using the respective  $M_S$  determined from SQUID measurements of the samples.

## RKKY COUPLING

### Anomalous Hall Effect Measurements

The sign of the interlayer exchange coupling in the multilayers was determined by separating the antiferromagnetic (AFM) and ferromagnetic (FM) coupling regimes of different Ir thicknesses. Anomalous Hall effect (AHE) measurements were performed in order to measure the saturation fields  $\mu_0 H_S$  of the different samples. In a cer-

tain thickness range, Ir induces AFM coupling via RKKY coupling between the layers which leads to an increased saturation field [6, 7]. Samples within the FM range should exhibit no effect on the saturation fields.

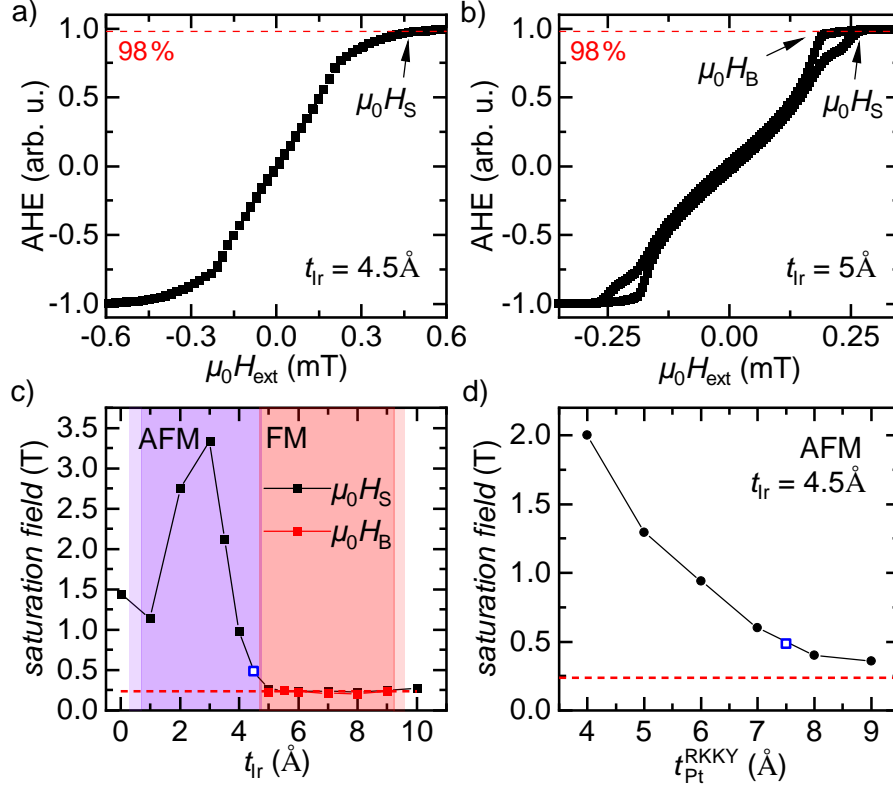

FIG. S4. a), b) Normalized anomalous Hall signal of the samples  $t_{\text{Ir}} = 4.5 \text{ \AA}$  and  $t_{\text{Ir}} = 5 \text{ \AA}$ . These two samples separate the two regimes with qualitatively different behavior in the hysteresis loops and thickness dependence of the saturation fields. For  $5 \text{ \AA} \leq t_{\text{Ir}} < 10 \text{ \AA}$ , hysteretic pockets close to  $\mu_0 H_S$  appear, whereas for  $t_{\text{Ir}} \leq 4.5 \text{ \AA}$ , hysteretic behavior is suppressed. The saturation field  $\mu_0 H_S$  is defined as the field necessary to saturate up to 98 %, whereas  $\mu_0 H_B$  is defined as the field at which saturation drops below 98 % coming from high fields. In c) the two distinct regions become evident, where  $\mu_0 H_S$  can be correlated with RKKY coupling. For low thicknesses, the interlayer exchange favors an antiparallel alignment (AFM coupling) which leads to an increase of the field necessary for saturation. When the coupling sign changes to a FM alignment, no effect on the saturation fields is visible. In this region,  $\mu_0 H_S$  stays constant at about 235 mT, indicated by the red line. The formation of the pockets is highlighted by adding  $\mu_0 H_B$  to the corresponding samples. d) The variation of Pt thickness with  $t_{\text{Ir}} = 4.5 \text{ \AA}$  shows AFM coupling behavior throughout all measured  $t_{\text{Pt}}$ . The blue square from c) is exported in d), perfectly matching the observed trend.

In Fig. S4 a) and b) we show the normalized AHE signal for two samples with  $t_{\text{Ir}} = 0.45 \text{ nm}$  and  $t_{\text{Ir}} = 0.5 \text{ nm}$ , which are representatives for the two qualitatively different hysteresis curves recorded. Some samples show no hysteresis, whereas others exhibit hysteresis loops close to saturation. The saturation field  $\mu_0 H_S$  is defined as the required field to saturate the sample up to 98 % and  $\mu_0 H_B$  represents the field at which saturation decreases below 98 % coming from higher fields. We see that a qualitative change takes place by changing the Ir thickness between  $t_{\text{Ir}} = 0.45 \text{ nm}$  and  $t_{\text{Ir}} = 0.5 \text{ nm}$ , indicative of two different coupling regimes. This becomes evident in Fig. S4 c), where the saturation and breakdown fields are plotted vs. the respective Ir thickness. Analogous to Karayev *et al.* [7], we observe a maximum  $\mu_0 H_S$  for a certain Ir thickness, and  $\mu_0 H_S$  drops drastically for higher or lower thicknesses. This behavior coincides well with the oscillation of RKKY coupling, indicating maximum, antiferromagnetic coupling strength at 0.3 nm Ir. When going above 0.45 nm, the RKKY coupling changes sign towards a ferromagnetic coupling, resulting in a constant saturation field. All ferromagnetically coupled multilayers share the commonality of forming hysteretic pockets, which allows discerning them qualitatively from AFM coupled samples.

A second sample series involves the variation of Pt thickness, where the Ir thickness is fixed in the antiferromagnetic regime close to its transition border. No qualitative change is observed in Fig. S4 d) within the range of values of  $t_{\text{Pt}}^{\text{RKKY}}$ , but a decay of antiferromagnetic coupling strength with increasing Pt thickness becomes evident. With help of this AHE sample study and by comparing the hysteresis curves, an antiferromagnetic RKKY coupling between

trilayers of the main text sample with  $t_{\text{Ir}} = 0.7 \text{ nm}$  and  $t_{\text{Pt}} = 0.6 \text{ nm}$  can be ruled out.

### Magnetic Force Microscopy

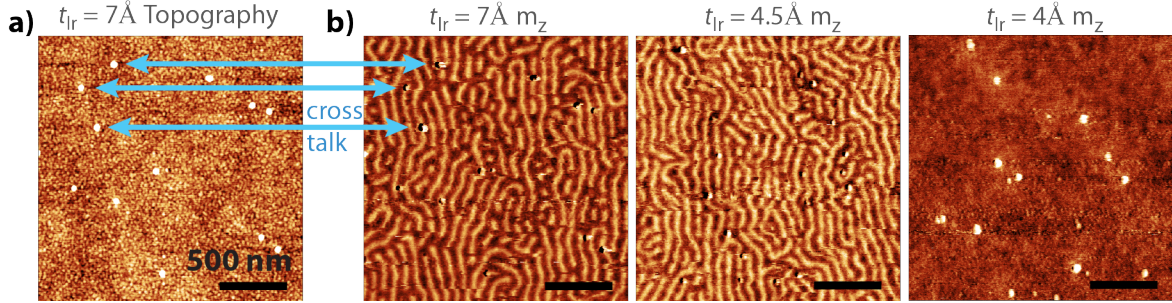

FIG. S5. a) Topography of the multilayer with Ir-thickness  $t_{\text{Ir}} = 7 \text{ Å}$  and its corresponding magnetic contrast in the first MFM image of b). Note, that the bright dots in b) are induced by cross talk from the topography and do not represent actual magnetic texture. The images show the domain formation in remanence for three multilayer samples with,  $t_{\text{Ir}} = 7 \text{ Å}$ ,  $4.5 \text{ Å}$ , and  $4 \text{ Å}$ . The thicknesses are chosen as representatives of ferromagnetic, weak AFM and stronger AFM coupling throughout the layers, respectively. In the first two images, a maze state is visible. Even though an AFM ordering would lead to compensating stray fields and, thus, vanishing magnetic contrast - as is the case in samples with  $t_{\text{Ir}} \leq 4 \text{ Å}$  - for the sample with  $t_{\text{Ir}} = 4.5 \text{ Å}$  small RKKY energies are overcome by dipolar contributions, resulting in labyrinthine domains. Hence, weak AFM and FM can not be distinguished from the remanent magnetic texture. The bright spots in the image of  $t_{\text{Ir}} = 4 \text{ Å}$  are related to topographical cross-talk and do not represent magnetic contrast.

Magnetic force microscopy was performed to identify the influence of the coupling sign on magnetic texture. In Fig. S5, the remanent state of three multilayer samples with different Ir-thicknesses ( $t_{\text{Ir}} = 7 \text{ Å}$ ,  $4.5 \text{ Å}$ ,  $4 \text{ Å}$ ) is shown. The chosen thicknesses work as representatives for FM, weak AFM, and stronger AFM coupling between the trilayers. In samples with  $t_{\text{Ir}} \leq 4 \text{ Å}$ , the moments align fully antiparallel and no MFM contrast is observed. The contrast changes drastically when weakening the AFM interaction. A labyrinthine state appears which looks similar to the maze state from the FM sample. This counterintuitive development of domains despite their coupling sign has been reported by Hellwig *et al.* and can be explained as a competition between RKKY and dipolar contributions [6]. Stripe domains

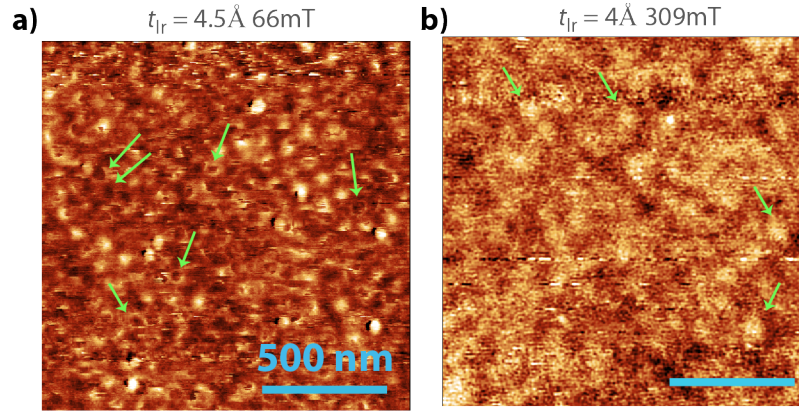

FIG. S6. Magnetic texture of the two AFM coupled samples with external applied magnetic fields. a) When applying fields to the weakly AFM coupled multilayer, the labyrinthine state decays into circular shaped domains, similar as in multilayers with FM coupling. Some circular domains (indicated by green arrows) look like "inverted" bubbles. b) For a sample with stronger AFM RKKY coupling and correspondingly strong AFM alignment in remanence, the canting due to external fields induces circular features, which become visible in the otherwise low magnetic contrast.

can form when dipolar interaction overcomes the negative RKKY interaction, such that a vertical, FM alignment throughout the layers is favored.

Similar to the images in the main text, circular shaped domains evolve, when applying magnetic fields in OOP direction to the AFM coupled samples. In Fig. S6 a) "popped" or "inverted" bubbles appear besides normal looking skyrmions. Some of them are marked by green arrows. Without further investigation, the magnetic texture is not clearly determined. Remarkably, the stronger coupled sample exhibits some circular shaped domains, although with very little contrast. Apparently, a canting of the AFM state - realized by external magnetic fields - enables skyrmion-like domain formation within these multilayers.

### MAGNETIC RESONANCE LINEWIDTH

Ferromagnetic resonance was used to determine the effective magnetization  $\mu_0 M_{\text{eff}}$  and quantify the damping of the multilayer. For this, we used a coplanar waveguide with a center width of  $w_{\text{CPW}} \approx 80 \mu\text{m}$ . The resonance field vs. frequency is plotted in Fig. S7 a), and fitted with the Kittel equation [8]:

$$\mu_0 H_{\text{res}} = \mu_0 M_{\text{eff}} + \frac{2\pi f}{\gamma} \quad (\text{S4})$$

where  $M_{\text{eff}} = M_{\text{S}} - H_{\text{k}}$  is the effective magnetization, and  $H_{\text{k}}$  is the uniaxial out-of-plane anisotropy field induced by the interface anisotropy.  $\gamma = g\mu_{\text{B}}/\hbar$  is the gyromagnetic ratio with the Landé factor  $g$ . Positive values of  $M_{\text{eff}}$  indicate easy-plane anisotropy, whereas negative values indicate PMA. Figure S7 b) depicts the FWHM linewidth vs. frequency from which the Gilbert damping parameter  $\alpha_{\text{G}}$  is determined by [9, 10]:

$$\mu_0 \Delta H = \mu_0 H_{\text{inh}} + 2 \cdot \frac{2\pi f \alpha_{\text{G}}}{\gamma}. \quad (\text{S5})$$

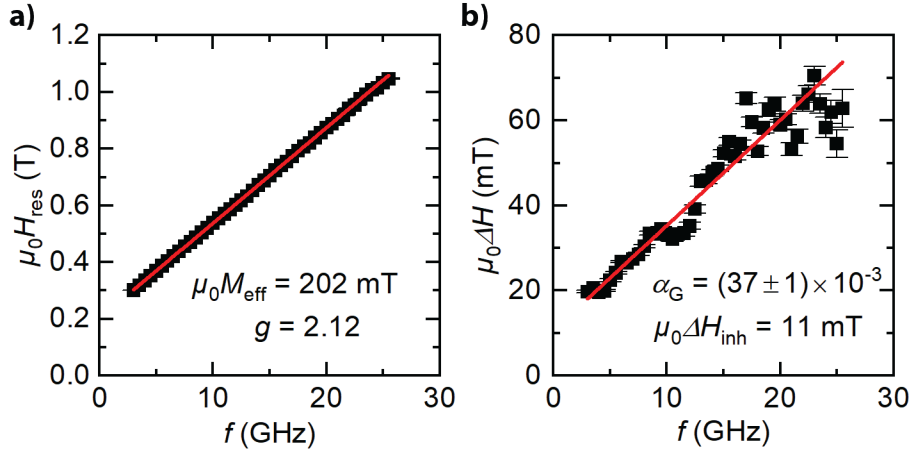

FIG. S7. Ferromagnetic resonance of the main sample. a) The resonance condition is fitted with the Kittel equation for thin films in OOP direction, such that  $M_{\text{eff}}$  and the Landé factor  $g$  can be extracted. b) Fits to the linewidth dependence on frequency are used to determine the Gilbert damping parameter  $\alpha_{\text{G}}$  and the inhomogeneous linewidth broadening  $\mu_0 \Delta H$ .

### MICROMAGNETIC SIMULATIONS

Both, dynamic and static response of the magnetic thin films were simulated using micromagnetic simulations [11] and compared to experimental results in Fig. S8. As, in our case, different exchange coupling values in the FM coupling regime seemed to have no significant effect on the hysteresis loops and domain sizes, simulations were carried out using a single layer film. A geometry of  $512 \times 512 \times 1$  cells with periodic boundary conditions was selected with cells of size  $3 \text{ nm} \times 3 \text{ nm} \times 12.6 \text{ nm}$ . Here, the lateral length of the cells is chosen to be smaller than the exchange length  $l_{\text{ex}} = \sqrt{2A/(\mu_0 M_{\text{S}}^2)} \approx 5.4 \text{ nm}$ , with values of  $A = 26 \text{ pJ/m}$  taken from literature [12] and  $M_{\text{S}} = 1212 \text{ kA/m}$

approximating the saturation magnetization determined from SQUID measurements. The thickness corresponds to 6 repetitions of 1.1 nm of FM layer and 1.0 nm of spacer material simulated as a single, effective ferromagnetic material. With an effective magnetization of  $\mu_0 M_{\text{eff}}^{\text{sim}} = 200$  mT, we obtain the first order uniaxial anisotropy constant  $K_u = 801.8$  kJ/m<sup>3</sup>. The DMI constant was set to  $D_{\text{int}} = 1.8$  mJ/m<sup>2</sup> and the Landé-factor  $g = 2.13$ .

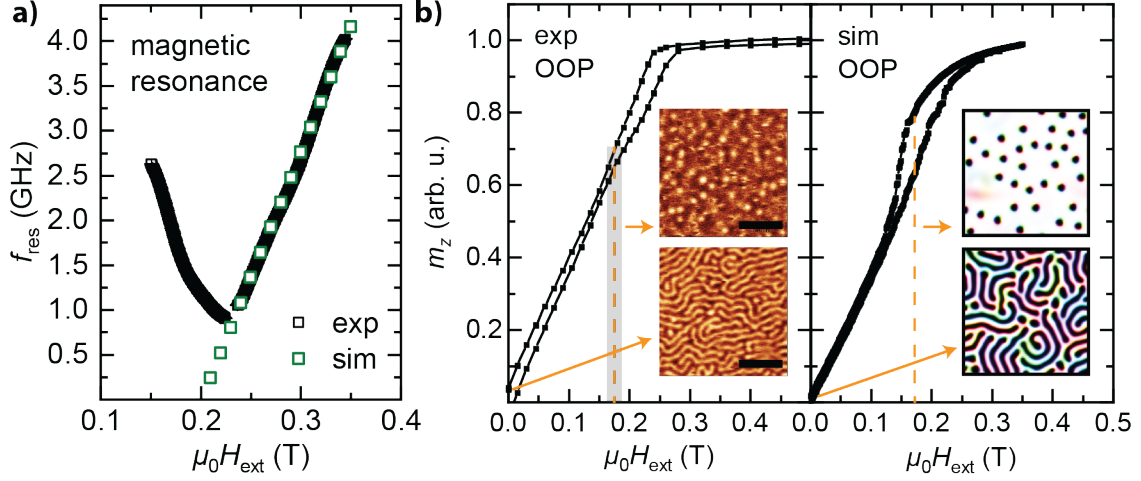

FIG. S8. Comparison of experimental data with simulations for dynamic and static investigations. a) The simulated eigenfrequencies of the simulated system match well the measured ferromagnetic resonance for  $\mu_0 H_{\text{ext}} \geq 240$  mT. b) The magnetization for different fields agrees well between measured SQUID data and micromagnetic simulations. MFM experiments and micromagnetic simulations show similar domains when increasing the applied field, as indicated by the respective insets. All insets depict images of  $1500 \text{ nm} \times 1500 \text{ nm}$  and the scale bar indicates 500 nm.

To obtain the FMR response, the sample was initialized at a small angle with the OOP axis and subsequently relaxed for decreasing static-external-field steps. At each field step, the equilibrium magnetization was excited using an additional external field with a sinc pulse in time and a homogenous spatial profile in the sample plane. Hysteresis curves have been obtained by initializing the magnetization in a random state at zero external field and then relaxing it at each step for increasing and subsequently decreasing field.

In Fig. S8 a), we see a very good agreement of the ferromagnetic resonance position extracted from the experiments and the simulations for large  $\mu_0 H_{\text{ext}}$ . However, the dynamic response below saturation could not be extracted from the simulations. The static response to external fields, shown in panel b), agrees qualitatively with the SQUID and MFM measurements. A hysteresis pocket is visible for fields slightly below saturation in simulation and experiment. At remanence, the labyrinthine domains form, which decay into a skyrmion state when applying OOP magnetic field. The existence of a skyrmion state is independent of the field history in simulations and experiment in accordance with skyrmion stabilization by DMI.

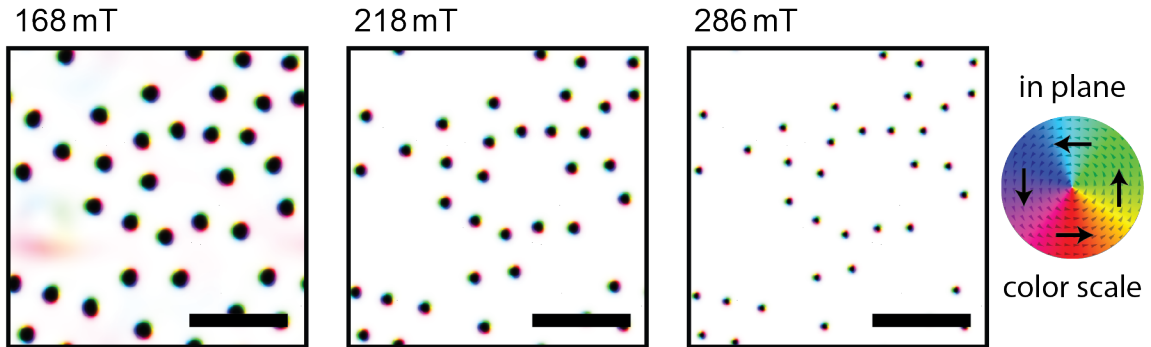

FIG. S9. The soliton size evolution shows a clear radius decrease with increasing fields, conforming with Zeeman energy contributions. Even though the environment captures the formation of skyrmions in a  $\mu_0 M_{\text{eff}} > 0$  system, the size stability could not be reproduced. The scale bar is 500 nm.

When comparing the domain size evolution of the simulations with the experimental data, another discrepancy

becomes evident. Although the analysis of the apparent radius from the MFM images yield a very stable skyrmion size for a large field range, micromagnetic simulations do not capture this feature of the easy-plane anisotropy skyrmion host. In Fig. S9, the soliton sizes at different applied external fields exhibit the typical shrinking with increasing fields, due to Zeeman energy. This indicates that a further anisotropy contribution which so far is not considered in our micromagnetic simulations is responsible for the experimentally observed behavior.

---

\* luis.flacke@wmi.badw.de

† weiler@physik.uni-kl.de

- [1] H. T. Nembach, J. M. Shaw, M. Weiler, E. Jué, and T. J. Silva, Linear relation between Heisenberg exchange and interfacial Dzyaloshinskii–Moriya interaction in metal films, *Nature Physics* **11**, 825 (2015).
- [2] K. Zeissler, M. Mruczkiewicz, S. Finizio, J. Raabe, P. M. Shepley, A. V. Sadovnikov, S. A. Nikitov, K. Fallon, S. McFadzean, S. McVitie, T. A. Moore, G. Burnell, and C. H. Marrows, Pinning and hysteresis in the field dependent diameter evolution of skyrmions in Pt/Co/Ir superlattice stacks, *Scientific Reports* **7**, 15125 (2017).
- [3] M. A. W. Schoen, D. Thonig, M. L. Schneider, T. J. Silva, H. T. Nembach, O. Eriksson, O. Karis, and J. M. Shaw, Ultra-low magnetic damping of a metallic ferromagnet, *Nature Physics* **12**, 839 (2016).
- [4] A. Soumyanarayanan, M. Raju, A. L. Gonzalez Oyarce, A. K. C. Tan, M.-Y. Im, A. P. Petrović, P. Ho, K. H. Khoo, M. Tran, C. K. Gan, F. Ernult, and C. Panagopoulos, Tunable room-temperature magnetic skyrmions in Ir/Fe/Co/Pt multilayers, *Nature Materials* **16**, 898 (2017).
- [5] J. Agustsson, U. Arnalds, A. Ingason, K. Gylfason, K. Johnsen, S. Olafsson, and J. Gudmundsson, Growth, coalescence, and electrical resistivity of thin Pt films grown by dc magnetron sputtering on SiO<sub>2</sub>, *Applied Surface Science* **254**, 7356 (2008).
- [6] O. Hellwig, A. Berger, J. B. Kortright, and E. E. Fullerton, Domain structure and magnetization reversal of antiferromagnetically coupled perpendicular anisotropy films, *Journal of Magnetism and Magnetic Materials* **319**, 13 (2007).
- [7] S. Karayev, P. D. Murray, D. Khadka, T. R. Thapaliya, K. Liu, and S. X. Huang, Interlayer exchange coupling in Pt/Co/Ru and Pt/Co/Ir superlattices, *Physical Review Materials* **3**, 041401 (2019).
- [8] C. Kittel, On the theory of ferromagnetic resonance absorption, *Physical Review* **73**, 155 (1948).
- [9] G. Woltersdorf, F. Hoffmann, H. G. Bauer, and C. H. Back, Magnetic homogeneity of the dynamic properties of (Ga,Mn)As films from the submicrometer to millimeter length scale, *Physical Review B* **87**, 054422 (2013).
- [10] R. D. McMichael, D. J. Twisselmann, and A. Kunz, Localized Ferromagnetic Resonance in Inhomogeneous Thin Films, *Physical Review Letters* **90**, 4 (2003).
- [11] A. Vansteenkiste, J. Leliaert, M. Dvornik, M. Helsen, F. Garcia-Sanchez, and B. Van Waeyenberge, The design and verification of MuMax3, *AIP Advances* **4**, 107133 (2014).
- [12] H. S. Körner, M. A. W. Schoen, T. Mayer, M. M. Decker, J. Stigloher, T. Weindler, T. N. G. Meier, M. Kronseder, and C. H. Back, Magnetic damping in poly-crystalline Co 25 Fe 75 : Ferromagnetic resonance vs. spin wave propagation experiments, *Applied Physics Letters* **111**, 132406 (2017).
